# Supplementary material for: Empir3D : A Framework for Multi-Dimensional Point Cloud Assessment
Source: arXiv:2306.03660 source file (2024-09-19)
Supplement: Supplementary file 1 [file suppl.tex]

% \documentclass[conference]{IEEEtran}
% \usepackage{times}
% \usepackage{soul}
% \usepackage{float}

% % numbers option provides compact numerical references in the text. 
% \usepackage[numbers]{natbib}
% \usepackage{multicol}
% \usepackage[bookmarks=true]{hyperref}



% \pdfinfo{
%    /Author (Yash Turkar)
%    /Title  (Empir3 : Point cloud assessment)
%    /CreationDate (D:20240202)
%    /Subject (Point cloud quality)
%    /Keywords (Point cloud;Perception; Benchmark)
% }

% %% Enable Comments
% % \newcommand{\rev}[1]{{\color{brown}Reviewer: #1}}
% \newcommand{\yash}[1]{{\color{orange}\large Yash: #1}}
% \newcommand{\pranay}[1]{{\color{blue}\large Pranay: #1}}
% \newcommand{\charu}[1]{{\color{green}\large Charu: #1}}
% \newcommand{\kar}[1]{{\color{red}\large KAR: #1}}
% \newcommand{\chris}[1]{{\color{purple}\large Chris: #1}}

% %% Disable Comments
% % \newcommand{\yash}[1]{}
% % \newcommand{\pranay}[1]{}
% % \newcommand{\charu}[1]{}
% % \newcommand{\kar}[1]{}
% % \newcommand{\chris}[1]{}
% % \newcommand{\rev}[1]{}



% % \newcommand{\tent}[1]{{\color{violet}#1}} % Tentative
% \newcommand{\verify}[1]{{\color{cyan}#1}} % Verify
% % \newcommand{\fixed}[1]{{\color{green}Fixed: #1}} % Fixed
% \newcommand\tent[1]{}
% % \newcommand\verify[1]{#1}
% % \newcommand\fixed[1]{}


% \newcommand{\qc}[1]{$Q_c$}
% \newcommand{\qa}[1]{$Q_a$}
% \newcommand{\qt}[1]{$Q_t$}
% \newcommand{\qr}[1]{$Q_r$}
% \newcommand{\qq}[1]{Empir3D}


% \newcommand{\cd}[1]{$D_{c}$}
% \newcommand{\hd}[1]{$D_{h}$}
% \newcommand{\emd}[1]{$D_{em}$}
% \newcommand{\dcd}[1]{$D_{dcd}$}


% % The following packages can be found on http:\\www.ctan.org
% \usepackage{graphicx} % for pdf, bitmapped graphics files
% %\usepackage{epsfig} % for postscript graphics files
% %\usepackage{mathptmx} % assumes new font selection scheme installed
% %\usepackage{times} % assumes new font selection scheme installed
% %\usepackage{amsmath} % assumes amsmath package installed
% %\usepackage{amssymb}  % assumes amsmath package installed
% \usepackage{multirow}
% \usepackage{multicol}
% \usepackage{array,booktabs}
% \usepackage[skins,theorems]{tcolorbox}

% \usepackage{tabularx}
% \usepackage{xcolor}
% % \usepackage{caption}
% \usepackage[font=small,labelfont=bf]{caption}
% \usepackage{subcaption}

% \usepackage{xr-hyper}
% \usepackage{hyperref}



% %% ----- Code to include refs from external docs ----- %%
% \makeatletter
% \newcommand*{\addFileDependency}[1]{% argument=file name and extension
% \typeout{(#1)}% latexmk will find this if $recorder=0
% % however, in that case, it will ignore #1 if it is a .aux or 
% % .pdf file etc and it exists! If it doesn't exist, it will appear 
% % in the list of dependents regardless)
% %
% % Write the following if you want it to appear in \listfiles 
% % --- although not really necessary and latexmk doesn't use this
% %
% \@addtofilelist{#1}
% %
% % latexmk will find this message if #1 doesn't exist (yet)
% \IfFileExists{#1}{}{\typeout{No file #1.}}
% }\makeatother

% \newcommand*{\myexternaldocument}[1]{%
% \externaldocument{#1}%
% \addFileDependency{#1.tex}%
% \addFileDependency{#1.aux}%
% }

% \myexternaldocument{paper-template-latex/root}

% %% ----- End code include refs from external docs ----- %%


% \begin{document}

% % paper title
% \title{\qq{} : A Framework for Multi-Dimensional Point Cloud Assessment\\
% \vspace{0.5cm}
% \large Supplementary Material}
% %\title{\qq{}: Evaluation Methodology for PoIntcloud Reasoning in 3D}

% % You will get a Paper-ID when submitting a pdf file to the conference system
% \author{}


% \maketitle
% % \begin{abstract}
    
% % \end{abstract}

% % \yash{Refer to sections in main papers as ~\autoref{related} in the main paper.} 

% The supplementary material extends the evaluation and discussion provided in the main manuscript. We show, in detail the efficacy and viability of using \qq{} as a general-purpose point cloud quality evaluation framework. The supplementary material is organized as follows, \autoref{suppl-eval-slam} has additional observations about the SLAM experiments in \autoref{eval_section} of the main paper including our method of collecting ground truth in the real world and the details about simulations, \autoref{suppl-eval-learning} demonstrates how \qq{} can be used in learning pipelines further and \autoref{suppl-eval-perf} describes the compute performance including memory and CPU utilization in details. Finally, in \autoref{suppl-appl} we discuss how \qq{} can be used example applications.

% \section{Evaluation}
% \label{suppl-eval-main}




% % \input{tables/slam_table_eps05_2}

% \subsection{Evaluation on Dense SLAM}
% \label{suppl-eval-slam}

% % \yash{I'm just dumping / describing now, everything will need some fixing - both in grammar and flow}

% % \subsubsection{Relationship between quantitative and qualitative results}
% % \yash{Check if there are too many repeating explanations compared to original}
% \autoref{warehouse_detailed} shows different views of the \emph{Warehouse} dataset, including magnified views for qualitative analysis. These images clearly show that SHINE and FAST-LIO2 significantly outperform LeGO-LOAM. \qq{} values corroborate with qualitative results by identifying SHINE's point cloud as the one with highest \qc{}, \qr{}, and \qa{} whereas \cd{} identifies FAST-LIO2. Of note, SHINE has a lower artifact-score (compared to FAST-LIO2) indicating the presence of artifacts, observed in \autoref{warehouse_detailed} where the pillars appear distorted due to artifacts. Further, \qq{} also accurately quantifies the lower resolution in LeGO-LOAM compared to others.

% \subsubsection{Constructing ground truth point clouds}
% % \yash{add image of surveying - some figure?}
% % \begin{figure}[ht]
% %   \centering
% %   % \vspace{-0.5cm}
% %   \includegraphics[trim=1cm 1cm 1cm 1cm, clip=true,width=\columnwidth]{supplm_images/Illuminati-gt-pose-map.pdf}
% %   \caption{Poses and point cloud for \emph{Davis} dataset}
% % \label{pose-map-davis}
% %   % \vspace{-10pt}
% % \end{figure}
% Acquiring ground truth for point cloud evaluation in a real-world setting is a challenging task. Although CAD and BIM files can be used, they're generally outdated and seldom represent the current environment. In outdoor settings, topographical maps and digital elevation models (DEMs) are sparse and lack rich 3D information.
% A common practice to build dense 3D models is the use of survey grade LiDAR scanners \citep{ARAYICI2007816,Mandlburger2023}, these use ground truth poses (from RTK GPS or Total-Stations) along with LiDAR scans to stitch a high-resolution 3D representation of the environment.

% We used a similar approach to build ground truth point clouds. First, we capture ground truth poses using a Robotic Total-Station \cite{kizil2011evaluation} which is essentially a theodolite with an integrated distance meter that can measure distances and angles. This enables extremely precise pose estimation (millimeter-level) and is widely used in infrastructure and geospatial surveying \cite{chekole2014surveying,totalstationtarvo}. Second, we capture LiDAR scans at the exact locations where poses are measured. This is achieved by placing a LiDAR mounted on a custom tripod, the tripod is equirped with a nadir pointed laser that projects a cross-hair onto carefully placed markers on the ground to align scans.
% For the \emph{Davis} dataset (\autoref{eval_section} in the main paper), over 400 poses (\autoref{pose-map-davis}) and corresponding scans were captured with this method. Finally, the scans are stitched into a dense point cloud of the environment with the recorded poses providing initial alignment. ICP was used for fine registration.
% \begin{figure}[H]
%   \centering
%   % \vspace{-0.5cm}
%   \includegraphics[trim=1cm 1cm 1cm 1cm, clip=true,width=\columnwidth]{supplm_images/Illuminati-gt-pose-map.pdf}
%   \caption{Poses and point cloud for \emph{Davis} dataset}
% \label{pose-map-davis}
%   % \vspace{-10pt}
% \end{figure}

% \begin{figure}[H]
%   \centering
%   % \vspace{-0.5cm}
%   \includegraphics[trim=1cm 1cm 1cm 1cm, clip=true,width=\columnwidth]{supplm_images/Sim-Worlds.pdf}
%   \caption{\emph{Warehouse} environment in simulation. Robot third-person view (left) and sensor output (right)}
% \label{sim-world}
%   % \vspace{-10pt}
% \end{figure}
% \begin{figure*}
%   \centering
%   % \vspace{-0.5cm}
%   \includegraphics[trim=1cm 1cm 1cm 1cm, clip=true,width=\textwidth]{supplm_images/Warehouse-Suppl2.pdf}
%   \caption{Evaluation on \emph{Warehouse} dataset (simulated);\ (a),(b),(c),(d) show point clouds ground truth, LeGO-LOAM, FAST-LIO2 and SHINE. (d) exhibits highest \qc{},\qa{},\qa{} as shown in zoomed-in view but contains artifacts (lower \qt{} compared to (c)). \qq{} accurately quantifies all aspects of quality while \cd{} and \hd{} identify (c) and (d) as the most similar}
% \label{warehouse_detailed}
%   % \vspace{-10pt}
% \end{figure*}
% \subsubsection{Simulation environment}
% % \yash{Add sim images - one of robot in sim and one of foxglove viz @christo}
% % \chris{I've added the images under supplm images}
% The simulator (\autoref{sim-world}) built to study \qq{}'s performance supports various environments, these are mesh files of objects and structures and can be built using popular tools like Blender ~\cite{blender}. The simulator supports three variants of the Ouster OS series LiDARs, namely the OS-0, OS-1 and OS-2 sensors. These allow a max vertical field-of-view of 90, 45 and 22.5 degrees respectively. Each of the sensor can be configured in three resolutions - 128, 64 and 32 channels. This totals to nine distinct LiDARs in simulation. We also add noise to simulate realistic outputs which can be tuned to match the sensor. Additionally, the simulator outputs IMU data and ground truth odometry for use in SLAM methods that need IMU or need external pose information.


% % \input{tables/learning_suppl}
% \begin{figure*}
%   \centering
%   % \vspace{-0.5cm}
%   % \includegraphics[trim=1cm 1cm 1cm 1cm, clip=true,width=\textwidth]{supplm_images/Completion_net_suppl.pdf}
%   \includegraphics[trim=1cm 1cm 1cm 1cm, clip=true,width=\textwidth]{supplm_images/suppl_learning_detailed.pdf}
%   \caption{Evaluation on point cloud completion, Lamp from MVP \cite{pan_variational_2021} reconstructed using PCN~\cite{yuan_pcn_2018}, TOPNET~\cite{tchapmi_topnet_2019}, ECG~\cite{pan_ecg_2020}. ECG generates highest quality point clouds which is confirmed by \qq{} metrics while \cd{} and \hd{} identify PCN despite presence of artifacts and poor reconstruction. \label{learning-detailed}}
%   % \vspace{-10pt}
% \end{figure*}


% \subsection{Evaluation on point cloud completion}\label{suppl-eval-learning}
% % \yash{Need to add learning table, figure and explain, dont think there is too much to disucss - @pranay }
% \autoref{learning-detailed} shows evaluation of point clouds generated using three point cloud completion networks, namely, PCN~\cite{yuan_pcn_2018}, TOPNET~\cite{tchapmi_topnet_2019} and ECG~\cite{pan_ecg_2020}. PCN and ECG output relatively high quality point clouds while TOPNET lags behind, producing noisy and incomplete results. These observations are corroborated by \qq{}'s metrics which denote ECG's output as the one with highest quality while \cd{} and \hd{} show PCN as the most similar. At the same time, \hd{} indicates lower similarity for ECG's point clouds contradicting visual observations and other metrics. This illustrates \cd{} and \hd{}'s limitations in quantitative quality evaluation.
% % \autoref{learning-detailed} shows results for different point cloud completion networks. \chris{Is this line relevant? The table is not present} Highlighted in bold in \autoref{learning_table_suppl}, ECG model outperforms in most of the categories which is captured by \cd{} as well as \qq{} metrics and corroborated qualitatively in \autoref{learning-detailed}. \qq{} metrics, however, give us further information where we see that ECG outperforms due to better accuracy and coverage. This could be beneficial to fine-tune the models to perform better, which cannot be attained by unbounded metric values like \cd{} and \hd{}.

% % \charu{Check if the following paragraph is required and/or cut down}
% % For Airplane model though \qc{}  of TOP-NET model is highest, but \qt{} score is lowest, while PCN as consistently high values in all the \qq{} metrics, ECG outperforms in accuracy which also can be corroborated by \autoref{slearning-detailed}. Additionally \cd{} also suggest ECG output as best. Similar results can be seen for Table model. Finally, a typical failure case of \cd{} can be seen for Lamp model, where though its value is least for PCN but \qq{} metrics suggest that ECG is best overall, which is clear in \autoref{learning-detailed}. The \hd{} is totally useless in learning output assessment as it do not indicate any model output performance consistently and indicating TOP-NET to be best, which contradicts with the visuals.
% % This further strengthen the value of \qq{} as a generalize metric to assess point cloud quality.


% \subsection{Compute Performance}
% \label{suppl-eval-perf}

% \begin{figure*}
%   \centering
%   % \vspace{-0.5cm}
%   % \includegraphics[trim=1cm 1cm 1cm 1cm, clip=true,width=\textwidth]{supplm_images/Completion_net_suppl.pdf}
%   \includegraphics[trim=1cm 1cm 1cm 1cm, clip=true,width=\textwidth]{supplm_images/Compute-Plots-RSS2.pdf}
%   \caption{Comparative analysis of memory, CPU utilization and computation time across different region sizes (r) and number of processor cores.1 Memory utilization remains relatively constant across various core counts, whereas CPU utilization increases with more cores, especially for smaller region sizes before decreasing again when regions become too large for multi-threading. Computation time decreases significantly with the increase in region size up to a certain point, beyond which the benefits plateau, as shown in the benchmarks for 1, 2, 4, and 8 core computation of \qq{}, compared to the baseline single-threaded implementations \cd{} and \hd{}.\label{compute-detailed}}
%   % \vspace{-10pt}
% \end{figure*}


% % \yash{running experiments for high region size - runtime should go up again showing a sweet spot, update writing accordingly}

% \qq{} compute performance is evaluated by calculating quality metrics for a sample point cloud. We compute \qq{} for a wide range of region sizes while \cd{} and \hd{} are calculated on the entire point clouds. Region sizes of {1, 2, 5, 10, 15, 20, 30, 50, 100} meters are chosen and run-time along with CPU and memory utilization is measured. Further, we repeat the experiments by limiting number of CPU cores for multi-threading providing some insights on computing on resource constrained hardware.

% Using \cd{} and \hd{} as baselines for reference, we observe that their CPU utilization is low and correspondingly the time taken to complete the evaluation is high.
% In contrast, our implementation of \qq{}, trades CPU utilization for execution time.
% In \autoref{compute-detailed}, we demonstrate this trade-off along with the effect of choosing different region sizes for parallelization on a benchmark point cloud.
% We observe that for smaller region size configuration, the CPU utilization is higher.
% As the region size is increased, the utilization dips as the region size grows closer to the size of the point cloud. 
% Eventually, \qq{}'s parallel implementation will reach a CPU utilization parity with \cd{} and \hd{} where entire point clouds are loaded on a single thread.

% On the other hand, we observe a trend in the execution time that might appear unusual at first glance. 
% The time taken by \qq{} starts to decrease with increase in region size but rises again for even higher values.
% We note that the reasons for this effect are two-fold. With much smaller region sizes, the individual region comparisons are quick. The major reason for this is that there are fewer points to consider for the closest point match. But, there are many regions to compute leading to a longer time. 
% As we increase the region size, the number of regions to compare reduces giving \qq{} a performance boost. At the same time, the time taken for the closest point search for individual regions increases.
% Finally, as the region size grows close to the full map, the time taken for closest point matches dominates leading to longer execution times. We hope that this analysis will help our readers make a judicious choice for the region size parameter for parallelization.
% Further, we note that as an added benefit of using lower region sizes is the lower memory usage.


% % \qq{} surpasses \cd{} and \hd{} in efficiency (run-time) while offering a richer analysis across various dimensions. As detailed in \autoref{compute-detailed} \yash{add sub fig refs}, the time required by \qq{} diminishes with increase in region sizes before increasing again for larger regions. 
% % The initial reduction is due to the decreased number of regions requiring computation, aided by its ability to effectively utilize multiple threads, which accelerates processing. 

% % Correspondingly, CPU utilization sees an increase with larger region sizes, as each region contains more points, demanding greater resources. The In case of memory usage, it remains relatively stable, as it primarily depends on the total size of the point clouds.
% % \yash{Next para on change in metrics with change in region size, I dont think they change , @christo check and add a plot of each metrics vs region size, we'll explain accordingly}
% % It is vital to note that region size minimally affects \qq{} evaluation as the primary goal is parallelized computation. We see this in \autoref{} where accuracy and resolution change by small margin with increase in region size while coverage and artifact-score do not. The former can be attributed to the fact that when \qq{} is evaluated over $N$ regions and averaged, the mean is not equal to what \qq{} will result in if computed over the whole point cloud. This only affects accuracy and resolution as they're computed as a function of point distances. \yash{@charu thoughts on previous sentence? I think this can be articulated better}

% \begin{figure}[ht]
%   \centering
%   % \vspace{-0.5cm}
%   \includegraphics[trim=1cm 1cm 1cm 1cm, clip=true,width=\columnwidth]{supplm_images/empir3d_metrics.png}
%   \caption{Plot shows change in \qq{} metrics with increase in region size ($r$). Resolution and accuracy are affected by averaging while coverage and artifact-score are not.}
% \label{region-qq}
%   % \vspace{-10pt}
% \end{figure}

% Since \qq{} metrics are averaged, a choice of region size will affect the actual values of some metrics (\autoref{region-qq}). While coverage and artifact-score are unaffected by region size, accuracy and resolution are affected by the averaging. However, this should not affect comparisons between different point clouds as long as the same region size is used for the comparisons.


% Region size affects CPU usage (thus time) and the memory usage. From our analysis, we make these recommendations:
% \begin{itemize}
%     \item Use lower regions sizes on memory constrained devices
%     \item Use higher region sizes in the order of map size on compute constrained devices
%     \item On unconstrained devices, use the region size to split the map into as many chunks in the order of the number of threads available on the device
% \end{itemize}


% %Region size can be chosen based on available compute resources and target application, \qq{} outputs metrics for each region giving detailed quality assessment of each region, this can be used to detect high and low quality areas in a point clouds. Ideally a smaller region size will provide high spatial fidelity when it comes to quality estimation at the cost of longer run-times. A sweet spot can be found where region size is 
% %\yash{Explain trade off - why a particular region size and how to pick one}


% \section{Applications and Use-cases}
% \label{suppl-appl}
% \begin{figure*}
%   \centering
%   % \vspace{-0.5cm}
%   \includegraphics[trim=1cm 1cm 1cm 1cm, clip=true,width=\textwidth]{supplm_images/Warehouse-Coverage.pdf}
%   \caption{Choosing sensors based on coverage and resolution; study shows \qq{} used to quantify performance of two LiDARs, namely the Ouster OS-0 and OS-1 128 channel. When \emph{Warehouse} environment is mapped using FAST-LIO2 with OS-0 the resulting point cloud exhibits higher overall coverage thanks to the increased vertical FOV while OS-1's point cloud is higher resolution increased vertical scan density.}
% \label{warehouse_coverage}
%   % \vspace{-10pt}
% \end{figure*}

% To illustrate \qq{}'s usage, consider the problem of selecting a suitable LiDAR sensor for dense mapping. 
% %We demonstrate in a study how this can be used to decide between two LiDAR sensors with varying vertical field-of-view (V-FOV) and range. 
% Given Ouster OS-0 and OS-1 LiDARs, with vertical FOV of 90 and 45 degrees respectively, a range of 35m and 90m respectively and a vertical resolution of 128 channels, we simulate both sensors in our simulator (\autoref{sim-world}) and map the \emph{Warehouse} environment using FAST-LIO2. 
% \autoref{warehouse_coverage} shows the point clouds and corresponding \qq{} metrics. FAST-LIO2 with OS-0 generated $pcd_{OS-0}$ and OS-1 generated $pcd_{OS-1}$. 

% $pcd_{OS-0}$ has higher coverage at 90.5\% compared to 89.36\% in $pcd_{OS-1}$, this is primarily due to the larger V-FOV of the OS-0 LiDAR. $pcd_{OS-1}$ on the other hand, has higher resolution at 97.86\% compared to 95.02\% in $pcd_{OS-0}$, this can be attributed to the spreading out of the 128 available vertical channels over different FOVs that produce different densities. Results indicate that the OS-1 is a better choice in this case due to the higher resolution in the maps despite the expanded coverage of OS-0.
% % \yash{also mention artifacts above}


% % \yash{Fix next para - does the last quant. relation make sense}
% This style of assessment can help pick sensors and algorithms based on expected coverage and resolution. Higher coverage and resolution generally results in improved SLAM performance, both in localization and mapping. This is because an increase in these metrics indicates an increase the number of features detected in the point cloud. To demonstrate this further, we compute ISS features \cite{zhong2009intrinsic} on both $pcd_{OS-0}$ and $pcd_{OS-1}$. $pcd_{OS-0}$ contains 1,531,103 features while $pcd_{OS-1}$ contains 1,509,107, this confirms the hypothesis that an increase of 1.14\% in coverage results in 1.45\% increase in the number of points detected.

% % \yash{One sentence to conclude and wrap up this section}

% % \section{Discussion}
% % \label{suppl-discuss}

% % \yash{Address ICRA comments}
% % \yash{

% % \begin{itemize}
% %     \item "for the evaluate in table II, it's unclear what the reader
% % is supposed to learn from it. Are the metrics successful?
% % If we know what different priorities we may have, do they
% % tell us which algorithm to use?"

% % \item " It seems like an uphill battle to convince people to switch
% % to using four metrics to evaluate point clouds rather than
% % the single number they are currently using"


% % \item "How do we evaluate equation 5 and 6 if the acquired map has
% % extra coverage compared to the ground truth map as we have
% % in Figure 4." ------- Need to mention that we take a total of both point clouds and then break into regions
% % \end{itemize}
% % }


% % \yash{Comment on combining metrics - examples; learning, coverage etc ..}

% % \yash{Not sure if we time for fault tolerance}

% \IEEEpeerreviewmaketitle

% \bibliographystyle{plainnat}
% \bibliography{paper-template-latex/filtered,paper-template-latex/additional}

% \end{document}
